# Supplementary material for: Transport in polymer membranes beyond linear response: Controlling permselectivity by the driving force
Source: arXiv:2106.05507 source file (2021-06-10)
Supplement: Supplementary file 1 [file SI.pdf]

# Supplemental Material — Transport in polymer membranes beyond linear response: Controlling permselectivity by the driving force

Won Kyu Kim,<sup>1,\*</sup> Sebastian Milster,<sup>2,3</sup> Rafael Roa,<sup>4</sup> Matej Kanduč,<sup>5</sup> and Joachim Dzubiella<sup>2,3,6,†</sup>

<sup>1</sup>*Korea Institute for Advanced Study, Seoul 02455, Republic of Korea*

<sup>2</sup>*Research Group for Simulations of Energy Materials,  
Helmholtz-Zentrum Berlin für Materialien und Energie, D-14109 Berlin, Germany*

<sup>3</sup>*Applied Theoretical Physics-Computational Physics, Physikalisches Institut,  
Albert-Ludwigs-Universität Freiburg, D-79104 Freiburg, Germany*

<sup>4</sup>*Departamento de Física Aplicada I, Facultad de Ciencias, Universidad de Málaga, E-29071 Málaga, Spain*

<sup>5</sup>*Jožef Stefan Institute, SI-1000 Ljubljana, Slovenia*

<sup>6</sup>*Cluster of Excellence livMatS @ FIT - Freiburg Center for Interactive Materials and Bioinspired Technologies,  
Albert-Ludwigs-Universität Freiburg, D-79110 Freiburg, Germany*

(Dated: June 4, 2021)

## I. PENETRANT CONCENTRATION, LONGITUDINAL VELOCITY, AND FLUX

The production run simulations were carried out for a sufficiently long time (several  $10^8$  time steps) to ensure the steady state (constant flux along the longitudinal  $z$  direction), for several different values of the fixed driving forces in each trajectory.

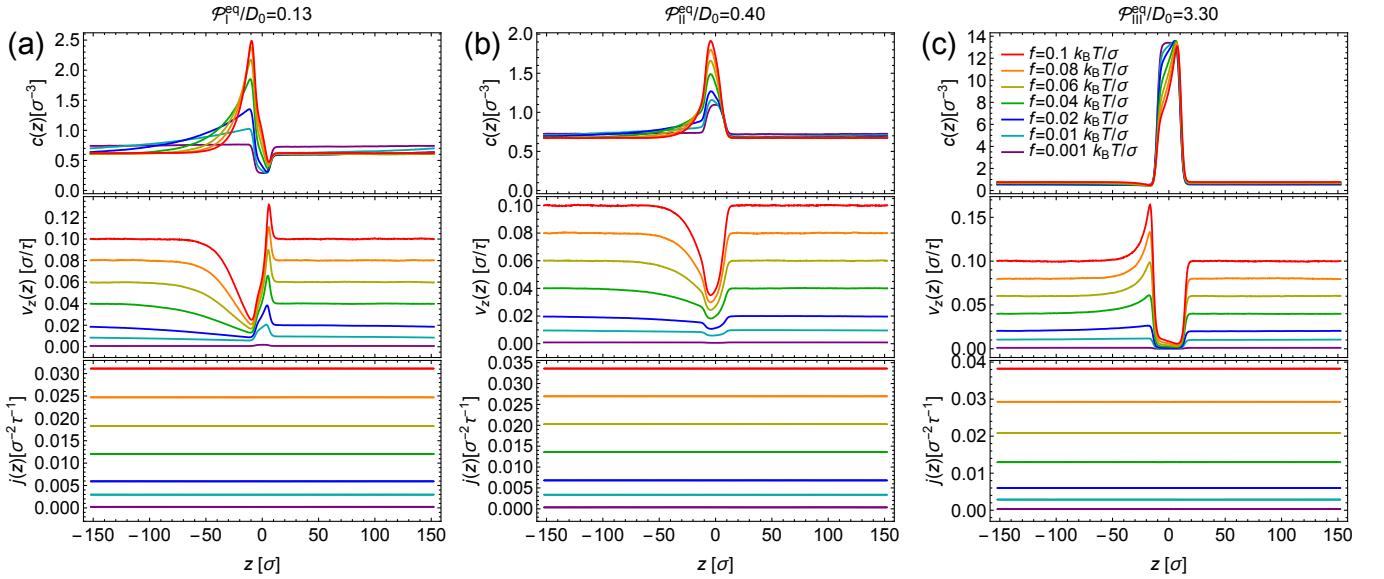

FIG. S1: Simulation results from the one-component penetrant system under the different external driving forces  $f$ , for (a)  $\epsilon_{np} = 0.1 k_B T$  and  $\mathcal{P}_I^{eq}/D_0 = 0.13$ , (b)  $\epsilon_{np} = 0.6 k_B T$  and  $\mathcal{P}_{II}^{eq}/D_0 = 0.40$ , and (c)  $\epsilon_{np} = 1.2 k_B T$  and  $\mathcal{P}_{III}^{eq}/D_0 = 3.30$ . Top panels: time-averaged steady-state concentration profiles of the penetrants  $c(z)$ . Middle panels: time-averaged steady-state velocity profiles of the penetrants  $v_z(z)$ . Bottom panels: time-averaged steady-state flux profiles of the penetrants  $j(z) = c(z)v_z(z)$ . The position  $z = 0$  corresponds to the center of the simulation box of length  $L$ . The equilibrium parameter values for  $\mathcal{P}^{eq}$  were taken from the force-free (equilibrium) simulations [1], and the fixed value of the solvent quality parameter (membrane interactions)  $\epsilon_{nn} = 0.5 k_B T$  was used.

\*Electronic address: wonkyukim@kias.re.kr

†Electronic address: joachim.dzubiella@physik.uni-freiburg.de

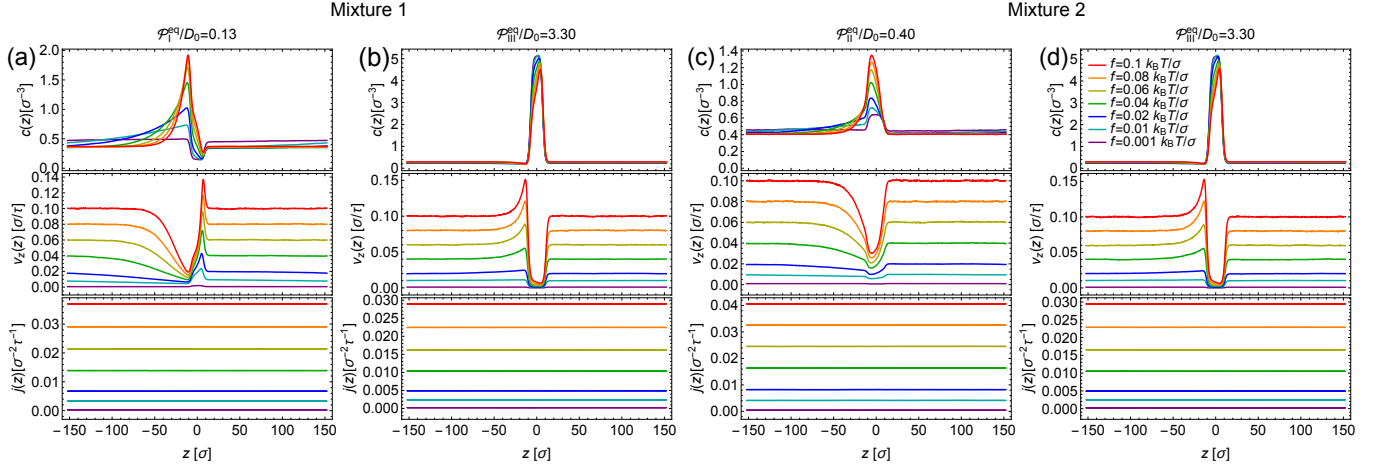

FIG. S2: Simulation results from the two-component mixtures under the different external driving force  $f$ , in Mixture 1: (a)  $\mathcal{P}_I^{\text{eq}}/D_0 = 0.13$ , (b)  $\mathcal{P}_{\text{III}}^{\text{eq}}/D_0 = 3.3$ , and Mixture 2: (c)  $\mathcal{P}_{\text{II}}^{\text{eq}}/D_0 = 0.4$ , (d)  $\mathcal{P}_{\text{III}}^{\text{eq}}/D_0 = 3.3$ . Top panels: time-averaged steady-state concentration profiles of the penetrants  $c(z)$ . Middle panels: time-averaged steady-state velocity profiles of the penetrants  $v_z(z)$ . Bottom panels: time-averaged steady-state flux profiles of the penetrants  $j(z) = c(z)v_z(z)$ . The position  $z = 0$  corresponds to the center of the simulation box length  $L$ . The equilibrium parameter values for  $\mathcal{P}^{\text{eq}}$  were taken from the force-free (equilibrium) simulations [1], and the fixed value of the solvent quality parameter (membrane interactions)  $\epsilon_{\text{nn}} = 0.5 k_B T$  was used.

In Fig. S1, we show the simulation results for the one-component penetrant systems. In the top panels, the time-averaged penetrant concentration profiles  $c(z)$  are depicted for different  $f$  (see the color legends in the panel c). In the middle panels, the time-averaged penetrant velocity profiles  $v_z(z)$  are depicted. In the bottom panels, the time-averaged penetrant flux profiles  $j(z) = c(z)v_z(z)$  are depicted, which are independent of  $z$ , i.e., in the steady-state.

In addition, we show in Fig. S2 the simulation results for the two-component mixtures, in the similar manner as shown in Fig. S1, which also exhibits the constant flux throughout the  $z$  direction.

---

[1] W. K. Kim, R. Chudoba, S. Milster, R. Roa, M. Kanduč, and J. Dzubiella, *Soft Matter* **16**, 8144 (2020).
